# Supplementary material for: Same or Not? Enhancing Visual Perception in Vision-Language Models
Source: arXiv:2512.23592 source file (2026-02-04)

## FQGVA (Pair)

**TWIN-Eval**

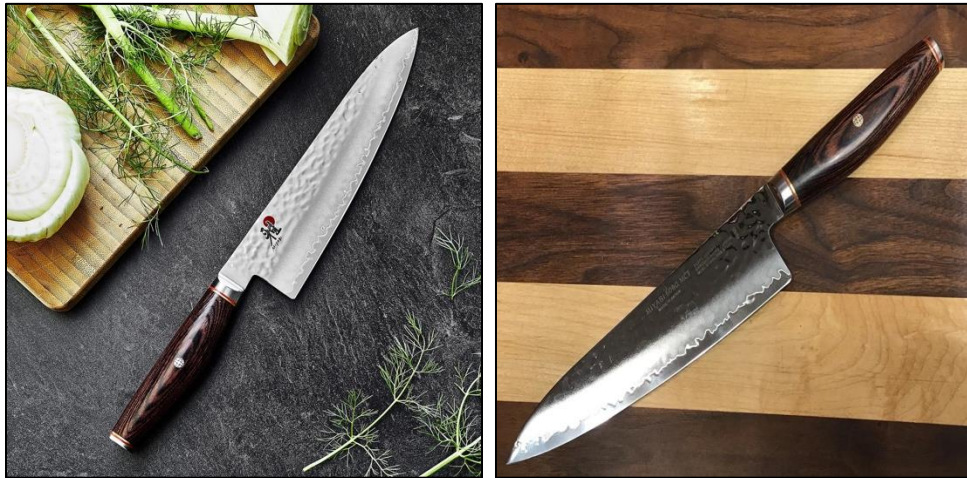

**Inquire**

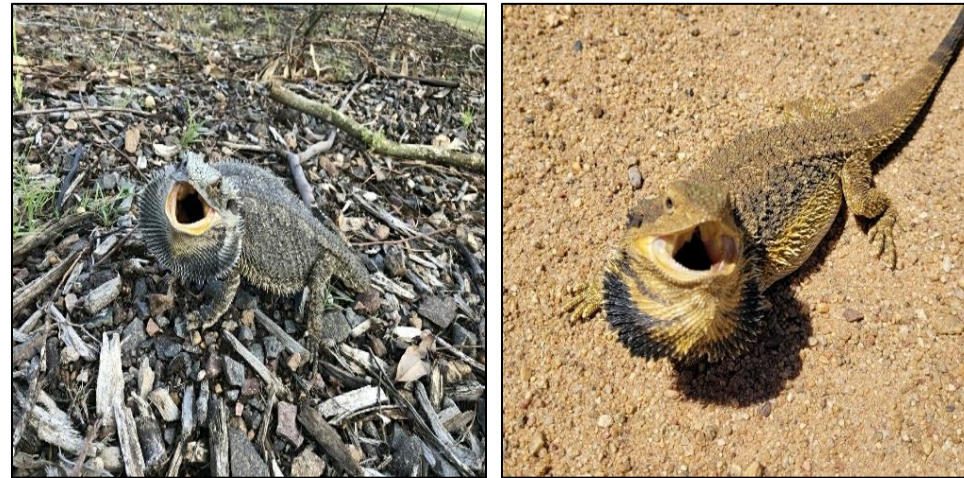

**Landmarks**

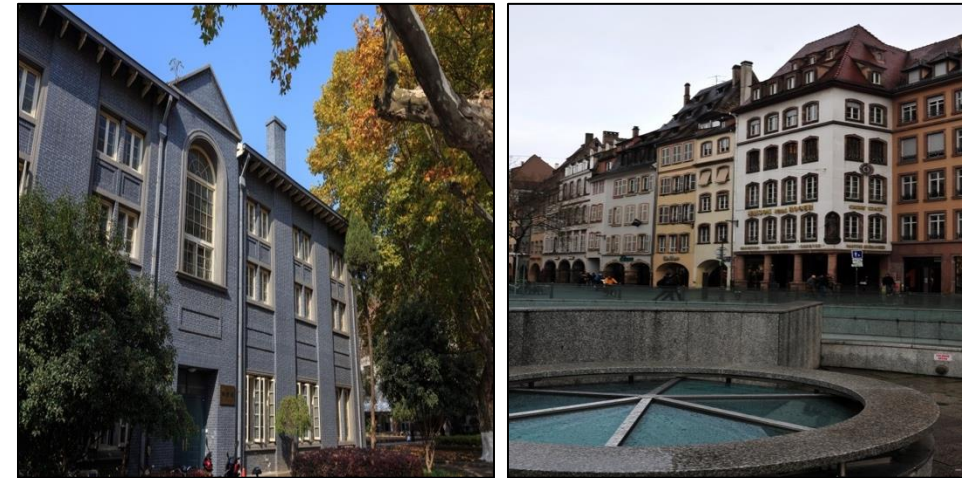

**CUB**

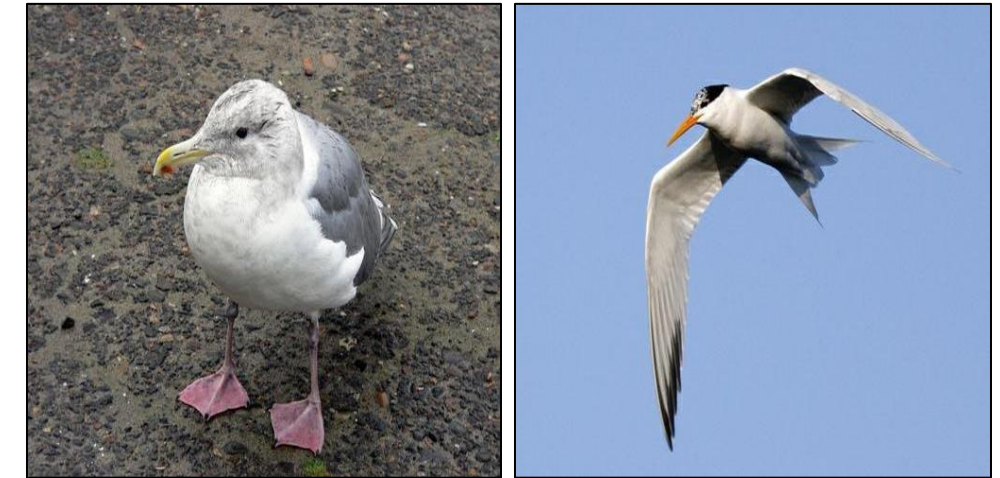

**Landmarks**

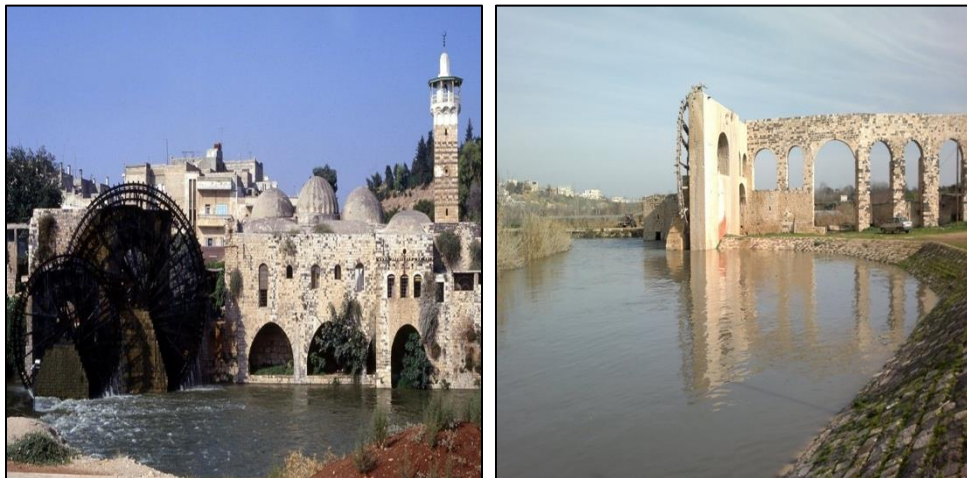

**MET**

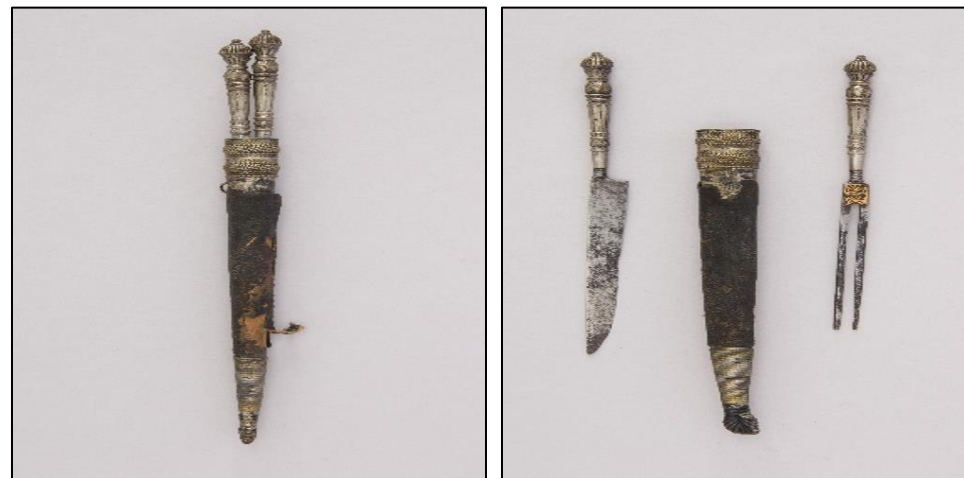

**TWIN-Eval**

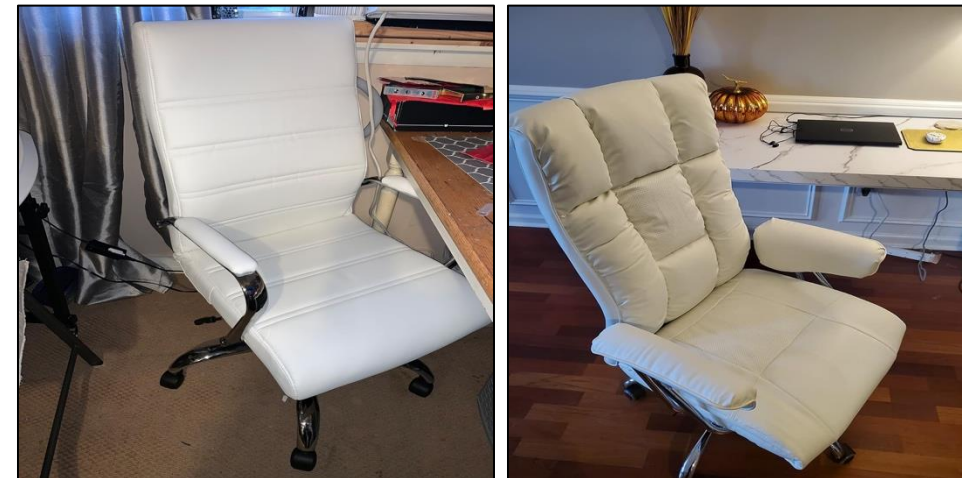

**Inquire**

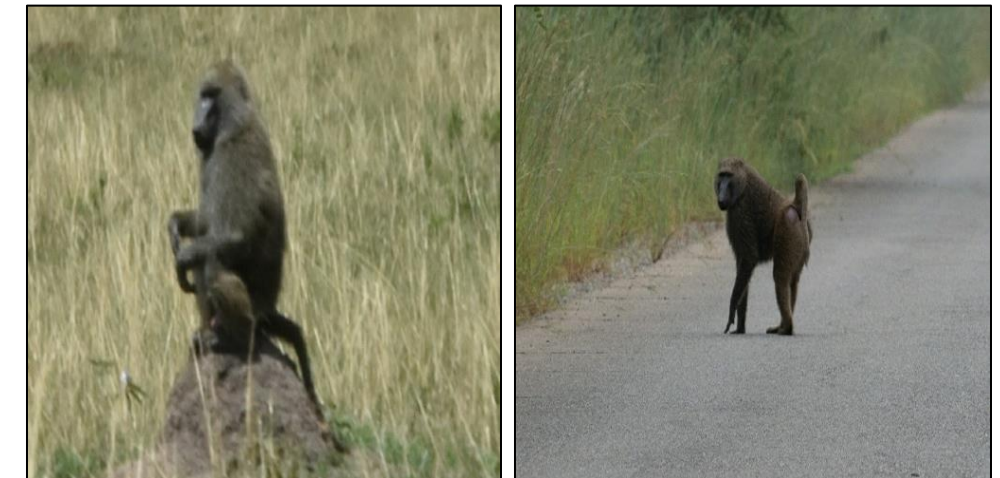

**MET**

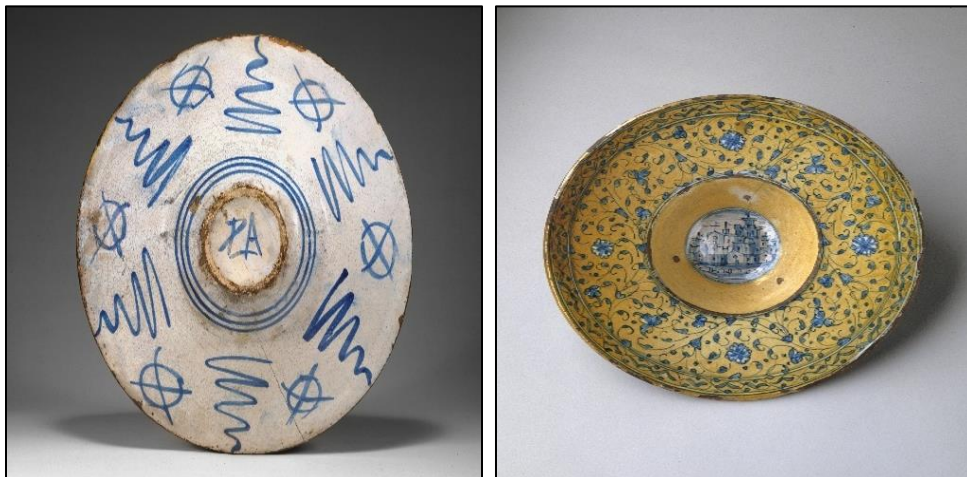

**CUB**

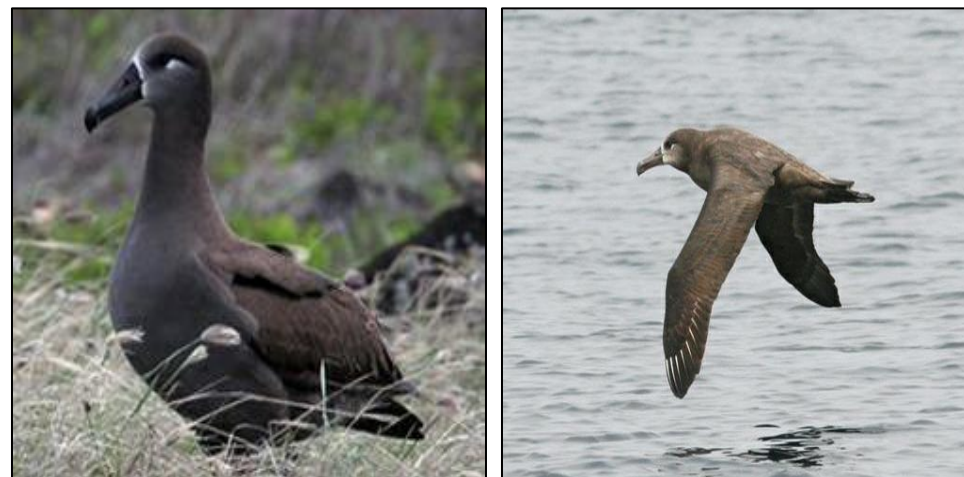

**TWIN-Eval**

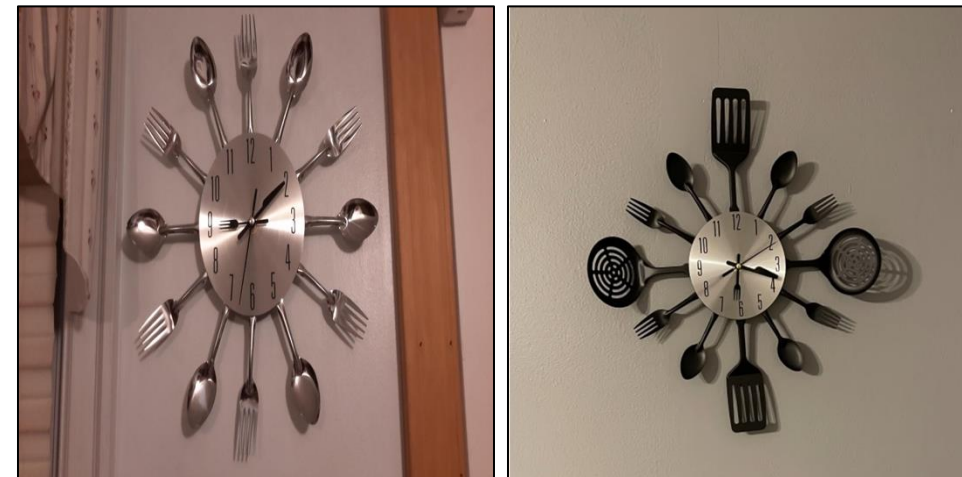

**ILIAS**

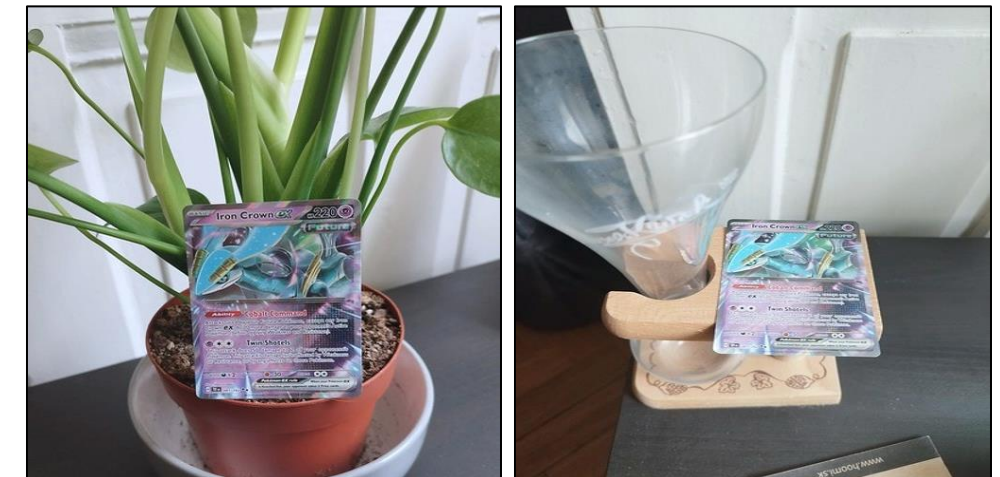

## FQGVA (Multi)

**TWIN-Eval**

**Reference**

**Image #1**

**Image #2**

**Image #3**

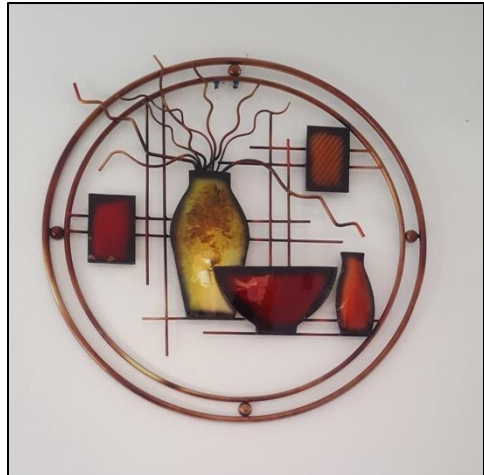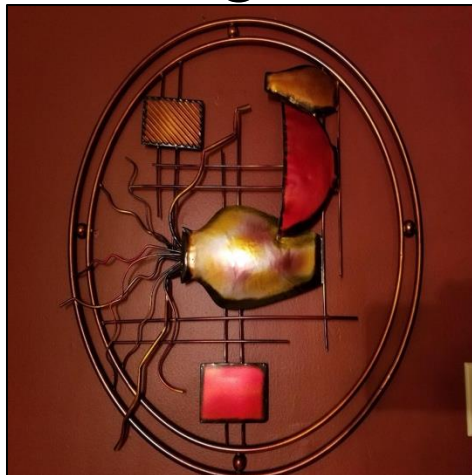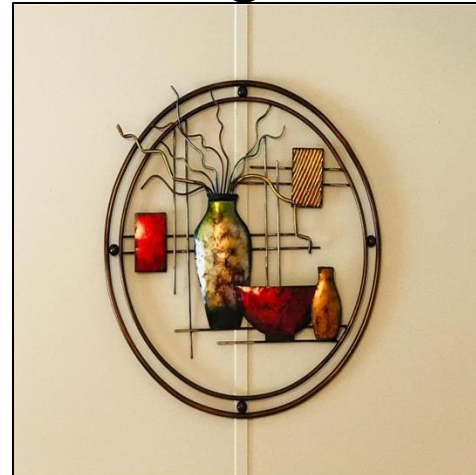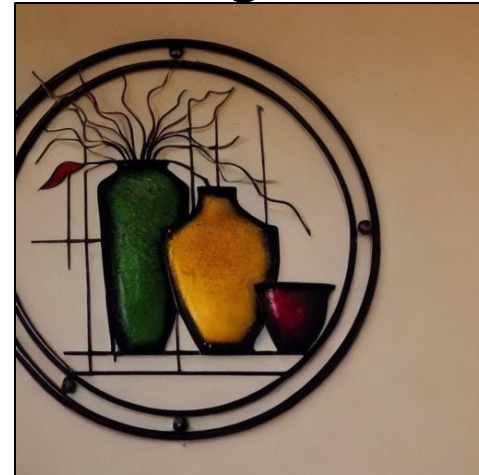

**Inquire**

**Reference**

**Image #1**

**Image #2**

**Image #3**

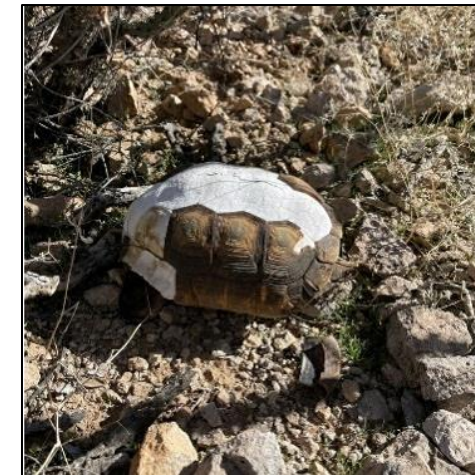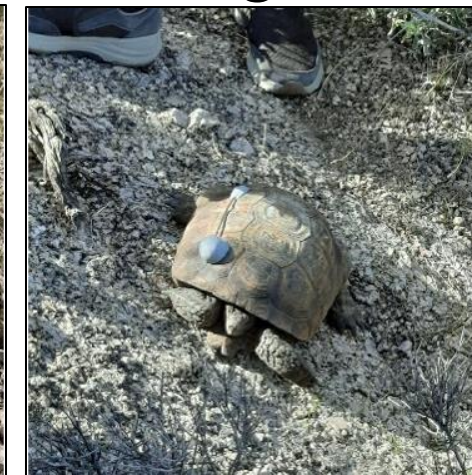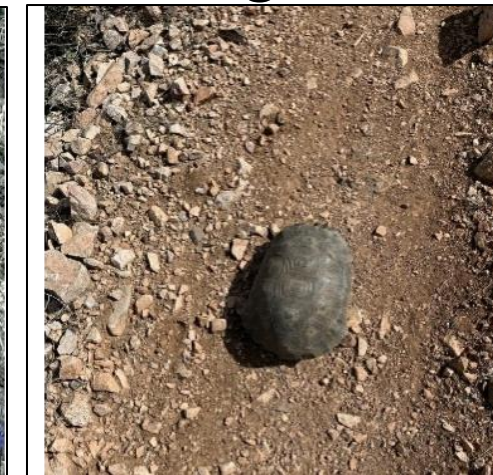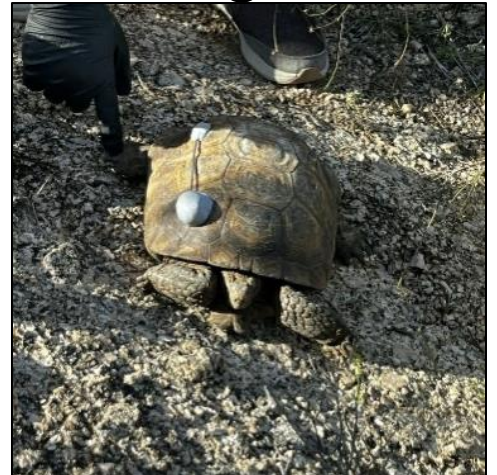

**Landmarks**

**Reference**

**Image #1**

**Image #2**

**Image #3**

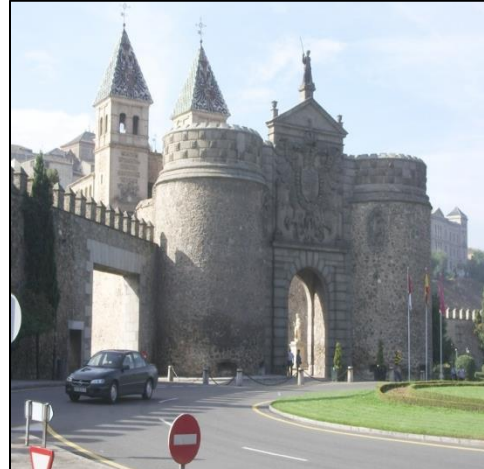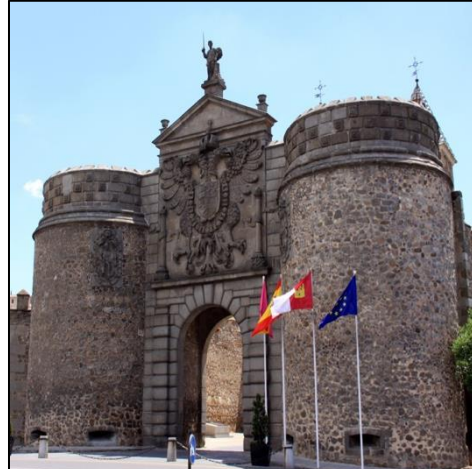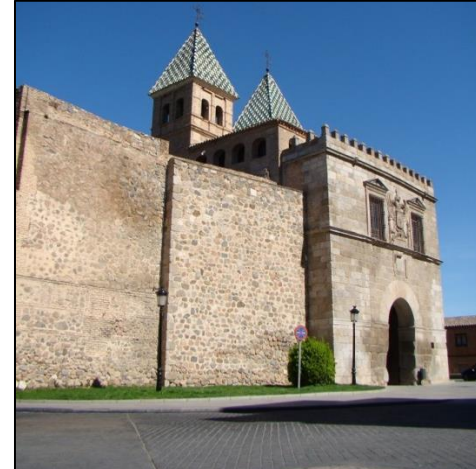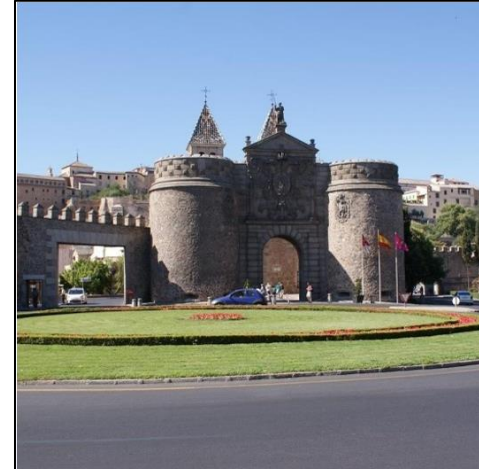

**CUB**

**Reference**

**Image #1**

**Image #2**

**Image #3**

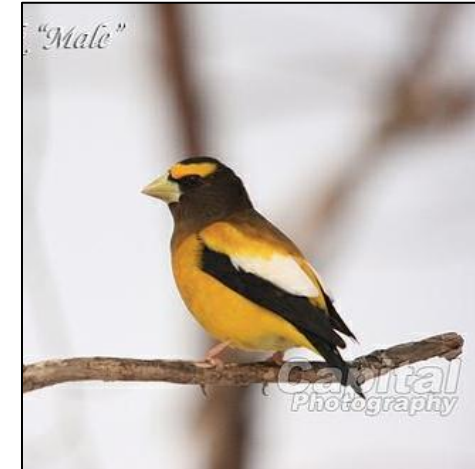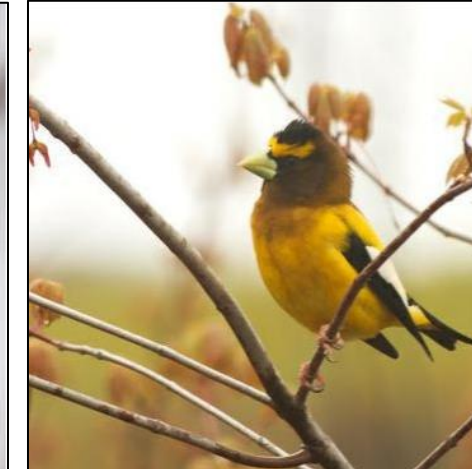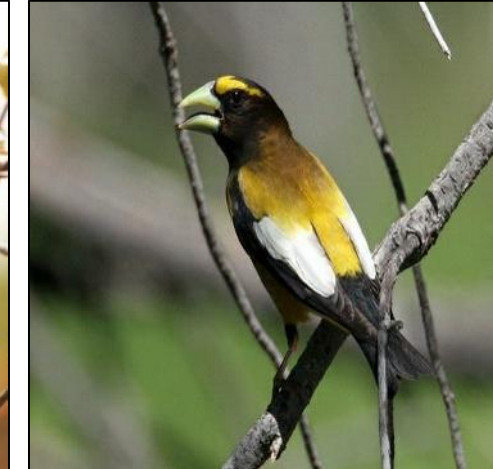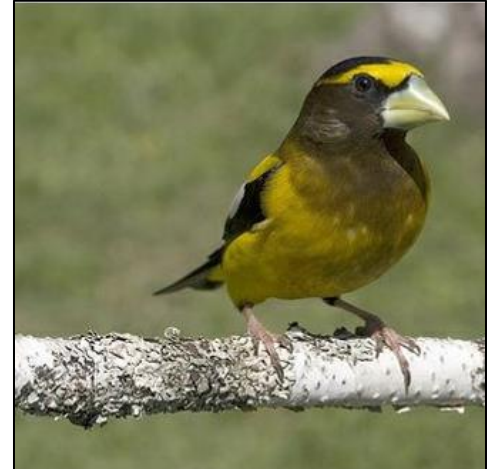

**ILIAS**

**Reference**

**Image #1**

**Image #2**

**Image #3**

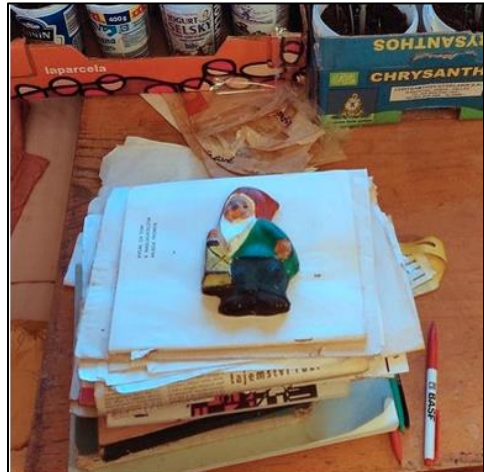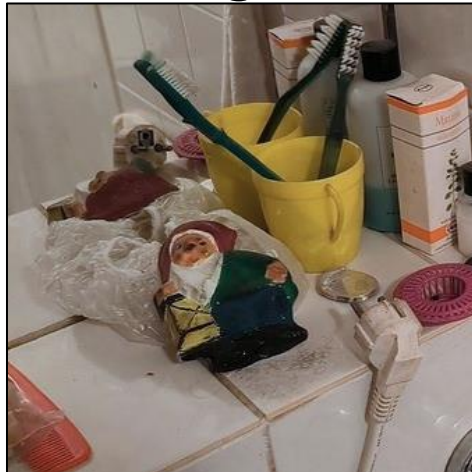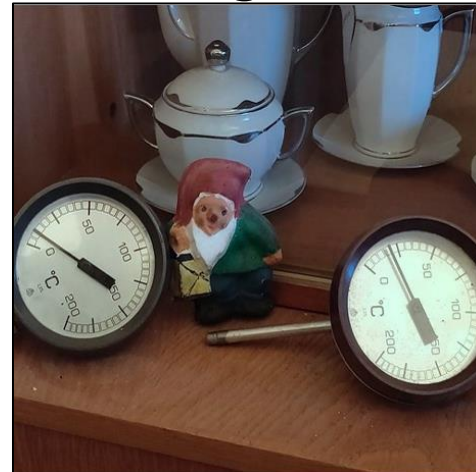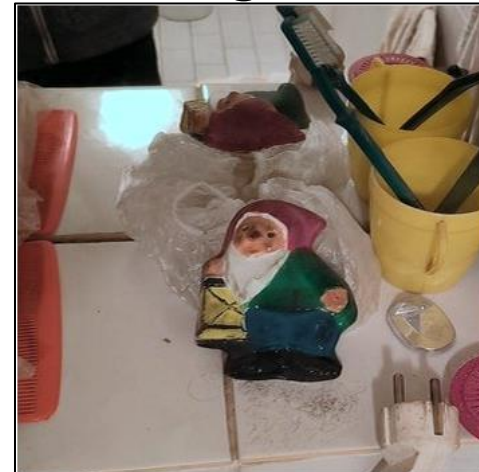

**MET**

**Reference**

**Image #1**

**Image #2**

**Image #3**

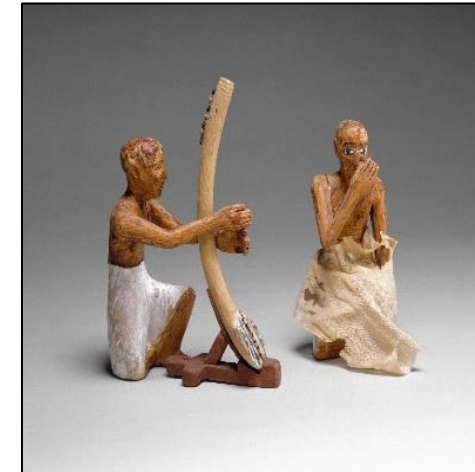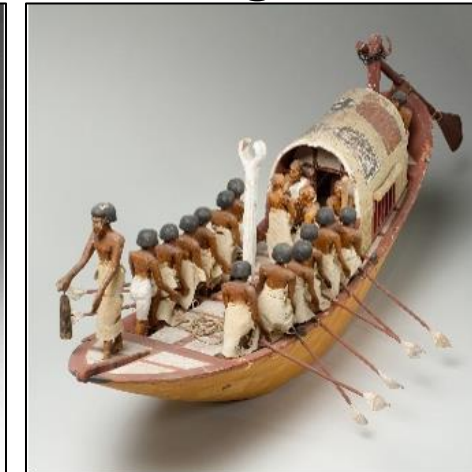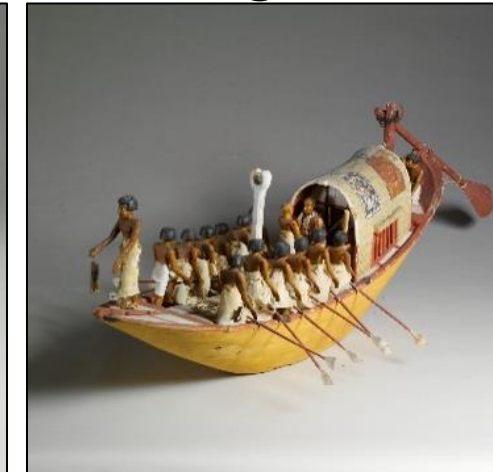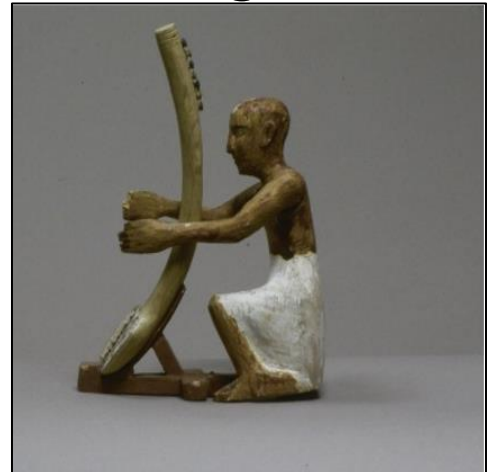



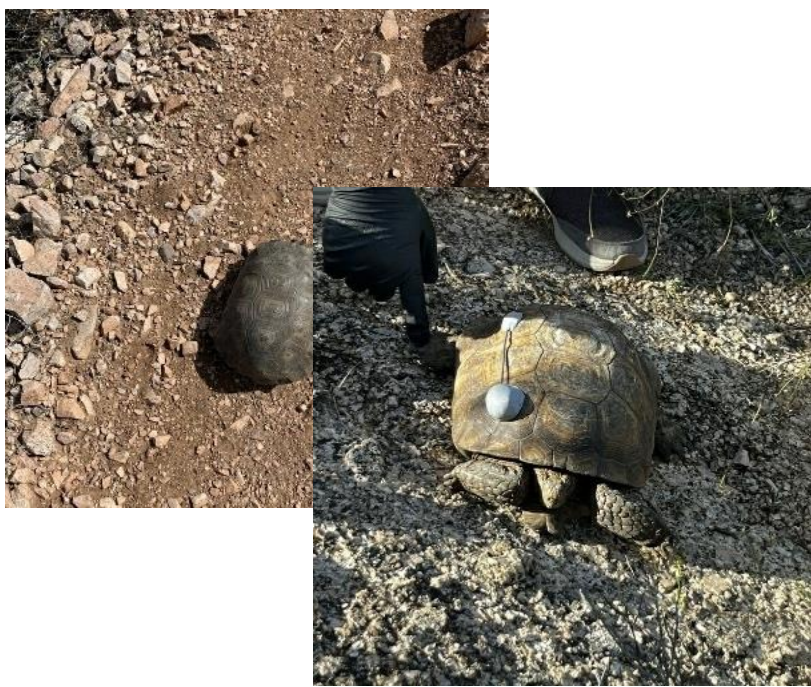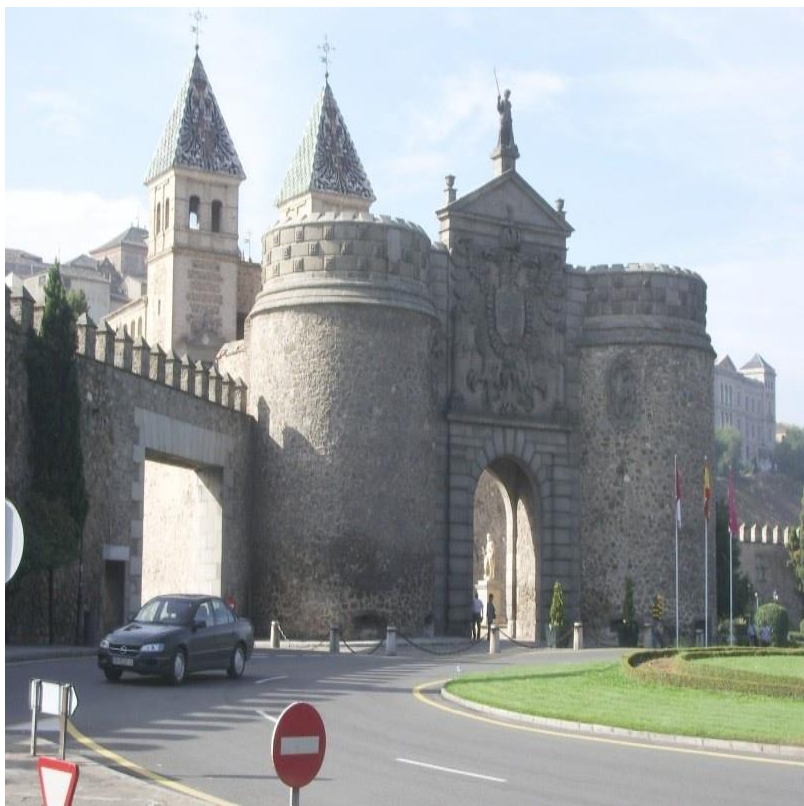

Supplement: Supplementary file 1 [file rao_supp_fgqva.pdf]
